# Supplementary material for: Poromechanical modelling of responsive hydrogel pumps
Source: arXiv:2503.01435 source file (2025-03-03)
Supplement: Supplementary file 1 [file supplementary_material.pdf]

# Poromechanical modelling of responsive hydrogel pumps

## Supplementary material

**Joseph J. Webber† and Thomas D. Montenegro-Johnson**
Mathematics Institute, University of Warwick, Coventry CV4 7AL, UK

## Modelling the swelling or shrinkage of hydrogel spheres in the LENS formalism

In order to validate the predictions of our model for thermo-responsive gels, we consider the swelling or drying of a gel with swollen equilibrium polymer fraction $\phi_{00}$, deswollen equilibrium polymer fraction $\phi_{0\infty}$ and radius $a_0$ when at swollen equilibrium. The polymer fraction evolution of a sphere which swells or dries axisymmetricaly (and hence has polymer volume fraction $\phi(r, t)$) follows the advection-diffusion equation

$$\frac{\partial \phi}{\partial t} + q_r \frac{\partial \phi}{\partial r} = \frac{1}{r^2}\frac{\partial}{\partial r}\left[r^2 D(\phi)\frac{\partial \phi}{\partial r}\right], \tag{S1}$$

where $D(\phi)$ is the nonlinear diffusivity. The phase-averaged flux $\boldsymbol{q} = q_r \hat{\boldsymbol{r}}$, and is solenoidal. This, coupled with the fact that $q_r = 0$ at the origin, sets $q_r \equiv 0$, so there is no advective contribution in this geometry. Conservation of polymer sets the evolution of the sphere radius, with

$$4\pi \int_0^{a(t)} r^2 \phi \, \mathrm{d}r = \frac{4\pi}{3} a_0^3 \phi_{00} \quad \text{so} \quad \frac{\mathrm{d}a}{\mathrm{d}t} = -\frac{D(\phi)}{\phi} \left.\frac{\partial \phi}{\partial r}\right|_{r=a(t)}, \tag{S2}$$

where we have differentiated the first equality with respect to time and substituted from equation (S1).

We consider the case of constant permeability $k$, and find the value of the material parameters $\mu_s(\phi)$ and $\pi(\phi)$ from the Gaussian-chain and Flory-Huggins formalisms, as deduced in the appendix. Together, these give a diffusivity

$$D(\phi) = \frac{k k_B T}{\mu_l \Omega_f}\left\{\frac{\phi - \phi^{1/3}/3}{\Omega} + \frac{\phi^2}{1-\phi} + 2\phi^2\left[\chi(\phi, T) + (1-2\phi)\frac{\partial \chi}{\partial \phi}\right] + \frac{4\phi^{1/3}}{3\Omega}\right\}. \tag{S3}$$

At the interface between gel and water, $r = a(t)$, continuity of pervadic pressure and normal stress together combine to show that osmotic pressures must be balanced by shear stresses. Thence, the polymer fraction here is given by $\phi = \phi_1$, with

$$\Pi(\phi_1) = 4\mu_s\left[\frac{a_0}{a(t)} - \left(\frac{\phi}{\phi_{00}}\right)^{1/3}\right]. \tag{S4}$$

At the origin, symmetry imposes $\partial\phi/\partial r = 0$. We then non-dimensionalise with $\Phi = \phi/\phi_{00}$, $A = a/a_0$, $R = r/a_0$ and $\tau = k k_B T t/\mu_l \Omega_f a_0^2$, and a non-dimensional diffusivity

$$\mathcal{D} = \frac{\phi - \phi^{1/3}/3}{\Omega} + \frac{\phi^2}{1-\phi} + 2\phi^2\left[\chi(\phi, T) + (1-2\phi)\frac{\partial \chi}{\partial \phi}\right] + \frac{4\phi^{1/3}}{3\Omega}. \tag{S5}$$

† Email address for correspondence: joe.webber@warwick.ac.uk

The full system of equations is therefore

$$\frac{\partial \Phi}{\partial \tau} = \frac{1}{R^2}\frac{\partial}{\partial R}\left[R^2 \mathcal{D}(\Phi)\frac{\partial \Phi}{\partial R}\right] \quad \text{with} \quad \Phi(A(\tau), \tau) = \Phi_1, \ \left.\frac{\partial \Phi}{\partial R}\right|_{R=0} = 0, \tag{S6a}$$

$$\frac{\phi_1 - \phi_1^{1/3}}{\Omega} - \phi_1 - \log(1-\phi_1) - \phi_1^2\chi + \phi_1^2(1-\phi_1)\frac{\partial \chi}{\partial \phi} = \frac{4\phi_{00}^{1/3}}{3\Omega}\left[\frac{1}{A(\tau)} - \left(\frac{\phi_1}{\phi_{00}}\right)^{1/3}\right], \tag{S6b}$$

$$\frac{\mathrm{d}A}{\mathrm{d}\tau} = -\frac{\mathcal{D}(\Phi)}{\Phi}\left.\frac{\partial \Phi}{\partial R}\right|_{R=A(\tau)}. \tag{S6c}$$

In Butler & Montenegro-Johnson (2022), smooth swelling and drying problems are considered with which we compare our model's predictions. Using the so-called HHT parameters of Hirotsu *et al.* (1987), we take our reference temperature $T_0 = 304\,\mathrm{K}$, which gives $\phi_{00} = 5.227 \times 10^{-2}$. To facilitate better comparison with the fully-nonlinear results, remark that the scalings used in Butler & Montenegro-Johnson (2022) are not identical to those that we have used above. The non-dimensional radius $r_{BMJ}$ is scaled with the fully-dry radius of the sphere and the non-dimensional time $t_{BMJ}$ is not equal to $\tau$, with

$$r_{BMJ} = \phi_{00}^{-1/3} R \approx 2.674R \quad \text{and} \quad t_{BMJ} = \frac{\phi_{00}^{2/3}\tau}{\Omega} \approx 9.93 \times 10^{-3}\tau. \tag{S7}$$

The two cases that we replicate in our modelling are the following:

(i) A swelling sphere where the temperature is lowered from 308 K to 304 K. Solving $\Pi(\phi) = 0$ at the higher temperature shows that $\phi_{0\infty} \approx 0.6425$, and so we solve the system (S6) with $\Phi(R, 0) \approx 12.29$ and $A(0) \approx 0.433$.

(ii) A drying sphere where the temperature is raised from 304 K to 307.6 K, so initial conditions are $\Phi(R, 0) = 1$ and $A(0) = 1$.

## REFERENCES

Butler, M. D. & Montenegro-Johnson, T. D. 2022 The swelling and shrinking of spherical thermo-responsive hydrogels. *J. Fluid Mech.* **947**, A11.

Hirotsu, S., Hirokawa, Y. & Tanaka, T. 1987 Volume-phase transitions of ionized N-isopropylacrylamide gels. *J. Chem. Phys.* **87** (2), 1392–1395.
